# Supplementary material for: Cluster detection in weak lensing surveys
Source: arXiv:0810.0781 source file (2008-10-06)
Supplement: Supplementary file 1 [file additional.tex]

In order to demonstrate our algorithm we use simulated weak lensing maps made 
from ray tracing through N-body simulations of structure formation
(\citet{white05}), covering $3 \times 3$ degree field of view. The cosmological 
model is taken to be a concordance $\Lambda$CDM model with parameters 
$\Omega_m=0.3$, $\Omega_{\Lambda}=0.8$, $\sigma_8=0.9$ and the Hubble parameter 
$h=0.7$. The simulations emplyed $384^3$ equal mass ($10^{10} M_{\sun} h^{-1}$) 
dark matter particles in a periodic cubical box of side $200 h^{-1} Mpc$ run
to $z=0$. The source redshift distribution was taken to be: 
\begin{equation}
p(z) \sim z^2 e^{-(z/z_0)^b}
\end{equation}
with $z_0=1.0$ and $b=1.5$.

The halo catalogue contains $563$ halos with $M_{200} > 5 \times 10^{13} 
h^{-1} M_{\sun}$ and redshifts between $0.0$ and $2.7$.

There are roughly $200$ galaxies per square arcminute in the simulation which
represents the deepest space-based surveys. In practice the signal-to-noise 
magnitude threshold gives around $100$ galaxies per square arcminute and then 
insisting on knowing the photo-z of each source pushes the number down to 
$40-70$ galaxies per square arcminute. Since there is no colour/magnitude
information for the sources available in these simulations, we pick $65$ 
galaxies per square arcminute randomly from the source catalogue. The intrinsic
ellipticity distribution of the source galaxies is assumed to be Gaussian with  
$\sigma_{int}=0.25$. We add Gaussian observational noise with standard 
deviation $\sigma_{obs}=0.20$ to the sheared ellipticity of each galaxy.

Modelling the whole $3 \times 3$ degree$^2$ field of view represents a highly
computationally expensive task and the MultiNest algorithm would require a
prohibitely large no. of live points to detect clusters with enough resolution.
We therefore divide the data in $16$ patches of $0.75 \times 0.75$ degree$^2$
each and use $3000$ live points to model each one of these $16$ patches. As
before, we expand the ranges of uniform priors on the position of cluster 
centers to allow them to lie a little outside their respective patches.
